# Supplementary material for: On Demographic Group Fairness Guarantees in Deep Learning
Source: arXiv:2412.20377 source file (2026-02-28)
Supplement: Supplementary file 1 [file suppl.tex]

\section{Appendix}
\label{sec:appendix}

\subsection{Proof of Theoretical Analysis}
\thmconnection*
\begin{proof}
First, we decompose the expected loss for each group into positive and negative components:

   \begin{align*}
   \mathbb{E}_{(x,y)\sim D_{a_k}}[\ell(f(x), y)] &= p_k \cdot L^{+,a_k}(f) + (1-p_k) \cdot L^{-,a_k}(f)
   \end{align*}

   for $k \in \{i, j\}$.

Now, consider the difference in expected losses:

   \begin{align*}
   &\left|\mathbb{E}_{(x,y)\sim D_{a_i}}[\ell(f(x), y)] - \mathbb{E}_{(x,y)\sim D_{a_j}}[\ell(f(x), y)]\right| \\
   &= \left|(p_i \cdot L^{+,a_i}(f) + (1-p_i) \cdot L^{-,a_i}(f)) - (p_j \cdot L^{+,a_j}(f) + (1-p_j) \cdot L^{-,a_j}(f))\right|
   \end{align*}

Rearrange the terms:

   \begin{align*}
   &= \left|p_i \cdot L^{+,a_i}(f) - p_j \cdot L^{+,a_j}(f) + (1-p_i) \cdot L^{-,a_i}(f) - (1-p_j) \cdot L^{-,a_j}(f)\right|
   \end{align*}

Add and subtract $p_i \cdot L^{+,a_j}(f)$ and $(1-p_j) \cdot L^{-,a_i}(f)$:

   \begin{align*}
   &= \left|p_i \cdot (L^{+,a_i}(f) - L^{+,a_j}(f)) + (p_i - p_j) \cdot L^{+,a_j}(f) \right. \\
   &\quad \left. + (1-p_j) \cdot (L^{-,a_i}(f) - L^{-,a_j}(f)) + (p_j - p_i) \cdot L^{-,a_i}(f)\right|
   \end{align*}

Apply the triangle inequality:

   \begin{align*}
   &\leq p_i \cdot \left|L^{+,a_i}(f) - L^{+,a_j}(f)\right| + |p_i - p_j| \cdot \left|L^{+,a_j}(f)\right| \\
   &\quad + (1-p_j) \cdot \left|L^{-,a_i}(f) - L^{-,a_j}(f)\right| + |p_j - p_i| \cdot \left|L^{-,a_i}(f)\right|
   \end{align*}

Note that $p_i \leq \max\{p_i, p_j\}$ and $(1-p_j) \leq \min\{1-p_i, 1-p_j\}$. Also, since $\ell$ is bounded by $M$, we have $\left|L^{+,a_j}(f)\right| \leq M$ and $\left|L^{-,a_i}(f)\right| \leq M$. Apply these bounds:

   \begin{align*}
   &\leq \max\{p_i, p_j\} \cdot \left|L^{+,a_i}(f) - L^{+,a_j}(f)\right| + M|p_i - p_j| \\
   &\quad + \min\{1-p_i, 1-p_j\} \cdot \left|L^{-,a_i}(f) - L^{-,a_j}(f)\right| + M|p_j - p_i|
   \end{align*}

We can simplify:

   \begin{align*}
   &\leq \max\{p_i, p_j\} \cdot \left|L^{+,a_i}(f) - L^{+,a_j}(f)\right| + 2M\left|p_i - p_j\right| \\
   &\quad + \min\{1-p_i, 1-p_j\} \cdot \left|L^{-,a_i}(f) - L^{-,a_j}(f)\right|
   \end{align*}

This completes the proof.
\end{proof}

% \begin{restatable}[Fairness Error Bound]{theorem}{thmfairerror}\label{thm:fair_errorbound}
% Under Assumption \ref{assm:prevalence}, given the fairness problem as defined in Definition \ref{eqn:def_fairness}, let $f^{*}$ be the optimal function that minimizes the maximum absolute difference in the expected loss across all demographic groups. Let $\hat{f}$ be an estimate of $f^{*}$ based on a finite sample of size $n$. Then, with probability at least $1 - \delta$, the following inequality holds:
% \begin{align*}
% &\max_{i, j} \left| \mathbb{E}_{(x, y) \sim \mathcal{D}_{a_i}}[\ell(\hat{f}(x), y)] - \mathbb{E}_{(x, y) \sim \mathcal{D}_{a_j}}[\ell(\hat{f}(x), y)] \right| \leq \\
% &\max_{i, j} \left| \mathbb{E}_{(x, y) \sim \mathcal{D}_{a_i}}[\ell(f^{*}(x), y)] - \mathbb{E}_{(x, y) \sim \mathcal{D}_{a_j}}[\ell(f^{*}(x), y)] \right| + M\sqrt{\frac{\log(2k/\delta)}{2n\min_{i}r_i}}
% \end{align*}
% \end{restatable}
\thmfairerror*
\begin{proof}
Let $L_i(f) = \mathbb{E}_{(x, y) \sim \mathcal{D}_{a_i}}[\ell(f(x), y)]$ be the expected loss for demographic group $a_i$ under function $f$. Define $\Delta(f) = \max_{i, j} |L_i(f) - L_j(f)|$ as the maximum absolute difference in the expected loss across all demographic groups.
\begin{lemma}[Hoeffding's Inequality for Bounded Loss]
For any function $f$ and demographic group $a_i$, with probability at least $1 - \delta_{i}$, the following inequality holds:
\begin{align*}
|L_i(f) - \hat{L}_i(f)| \leq M\sqrt{\frac{\log(2/\delta_{i})}{2n_{i}}}
\end{align*}
where $\hat{L}_i(f) = \frac{1}{n_{i}}\sum_{j=1}^{n_{i}} \ell(f(x_{j}^{(i)}), y_{j}^{(i)})$ is the empirical loss for group $a_i$, $n_{i} = nr_i$ is the sample size for group $a_i$, and $(x_{j}^{(i)}, y_{j}^{(i)})$ are i.i.d. samples from $\mathcal{D}_{a_i}$.
\end{lemma}
The lemma follows from Hoeffding's inequality and the fact that the loss function is bounded.
Applying the union bound and setting $\delta_{i} = \delta/k$ for all $i$, we have that with probability at least $1 - \delta$, the following inequality holds for all demographic groups simultaneously:
\begin{align*}
|L_i(f) - \hat{L}_i(f)| \leq M\sqrt{\frac{\log(2k/\delta)}{2n_{i}}} \leq M\sqrt{\frac{\log(2k/\delta)}{2n\min \{r_i\}}}
\end{align*}
Therefore, with probability at least $1 - \delta$, we have:
\begin{align*}
\Delta(\hat{f}) &\leq \Delta(f^{*}) + |\Delta(\hat{f}) - \Delta(f^{*})| \\
&\leq \Delta(f^{*}) + \max_{i, j} |L_i(\hat{f}) - L_j(\hat{f}) - (L_i(f^{*}) - L_j(f^{*}))| \\
&\leq \Delta(f^{*}) + \max_{i, j} (|L_i(\hat{f}) - \hat{L}_i(\hat{f})| + |L_j(\hat{f}) - \hat{L}_j(\hat{f})| + |L_i(f^{*}) - \hat{L}_i(f^{*})| + |L_j(f^{*}) - \hat{L}_j(f^{*})|) \\
&\leq \Delta(f^{*}) + 4M\sqrt{\frac{\log(2k/\delta)}{2n\min \{r_i\}}}
\end{align*}
This completes the proof.
\end{proof}
% -------------

% \begin{restatable}[Algorithmic Complexity of Fairness Problem]{theorem}{thmcomplexity}\label{thm:complexity}
% Under Assumption \ref{assm:Lipschitz}, given the fairness problem as defined in Definition \ref{eqn:def_fairness} with $k$ demographic groups and a function class $\mathcal{F}$ with finite Vapnik-Chervonenkis (VC) dimension $d$, there exists an algorithm that finds an $\epsilon$-optimal solution $\hat{f}$ to the fairness problem with probability at least $1 - \delta$, using $O(\frac{k^2}{\epsilon^2}(d\log(k/\epsilon) + \log(k/\delta)))$ samples and $O(k^2|\mathcal{F}|)$ time complexity.
% \end{restatable}
\thmcomplexity*
\begin{proof}
Let $f^{*} = \arg\min_{f \in \mathcal{F}} \Delta(f)$ be the optimal solution to the fairness problem, where $\Delta(f) = \max_{i, j} |L_i(f) - L_j(f)|$ is the maximum absolute difference in the expected loss across all demographic groups.
\begin{lemma}[Uniform Convergence Bound for Fairness Problem]\label{thm:convergence_bound}
Let $\mathcal{F}$ be a function class with finite VC dimension $d$. For any $\epsilon, \delta > 0$, if the sample size $n$ satisfies $n \geq \frac{8M^2k^2}{\epsilon^2}(d\log(16Mk/\epsilon) + \log(4k^2/\delta))$, then with probability at least $1 - \delta$, the following holds for all $f \in \mathcal{F}$ and all pairs of demographic groups $(i, j)$ simultaneously:
\begin{align*}
|L_i(f) - L_j(f) - (\hat{L}_i(f) - \hat{L}_j(f))| \leq \epsilon/2
\end{align*}
where $\hat{L}_i(f) = \frac{1}{n_i}\sum_{j=1}^{n_i} \ell(f(x_{j}^{(i)}), y_{j}^{(i)})$ is the empirical loss for group $a_i$, and $n_i = nr_i$ is the sample size for group $a_i$.
\end{lemma}
Lemma \ref{thm:convergence_bound} follows from the standard uniform convergence bound for finite VC dimension function classes, applied to the pairwise differences of the loss functions for each pair of demographic groups.
Now, consider the following algorithm:
\begin{enumerate}
    \item Draw a sample of size $n \geq \frac{8M^2k^2}{\epsilon^2}(d\log(16Mk/\epsilon) + \log(4k^2/\delta))$.
    \item For each $f \in \mathcal{F}$, calculate the empirical fairness error $\hat{\Delta}(f) = \max_{i, j} |\hat{L}_i(f) - \hat{L}_j(f)|$.
    \item Return $\hat{f} = \arg\min_{f \in \mathcal{F}} \hat{\Delta}(f)$.
\end{enumerate}

By Lemma \ref{thm:convergence_bound}, with probability at least $1 - \delta$, we have:
\begin{align*}
\Delta(\hat{f}) &\leq \hat{\Delta}(\hat{f}) + \epsilon/2 \\
&\leq \hat{\Delta}(f^{*}) + \epsilon/2 \\
&\leq \Delta(f^{*}) + \epsilon
\end{align*}
Therefore, the algorithm returns an $\epsilon$-optimal solution with probability at least $1 - \delta$. The sample complexity is $O(\frac{k^2}{\epsilon^2}(d\log(k/\epsilon) + \log(k/\delta)))$, and the time complexity is $O(k^2|\mathcal{F}|)$ since we need to calculate the empirical fairness error for each function in $\mathcal{F}$ and each pair of demographic groups.
\end{proof}

% -------------------

\begin{lemma}[Symmetrization]\label{thm:symmetrization}
For any function $f \in \mathcal{F}$,
\begin{align*}
\mathbb{P}\left[R(f) - R_{\text{emp}}(f) > \epsilon\right] \leq 2\mathbb{P}\left[\sup_{f \in \mathcal{F}} |R_{\text{emp}}(f) - R'{\text{emp}}(f)| > \frac{\epsilon}{2}\right]
\end{align*}
where $R(f)$ is the true fairness risk, $R_{\text{emp}}(f)$ is the empirical fairness risk on the original sample, and $R'_{\text{emp}}(f)$ is the empirical fairness risk on a ghost sample of size $m$ drawn independently from the same distribution as the original sample.
\end{lemma}
\begin{proof}
Let $S = {(x_1, y_1), \ldots, (x_m, y_m)}$ be the original sample of size $m$ and $S' = {(x'_1, y'_1), \ldots, (x'_m, y'_m)}$ be the ghost sample of size $m$, both drawn independently from the same distribution.
Define the event $A$ as:
\begin{align*}
A = {\exists f \in \mathcal{F}: R(f) - R_{\text{emp}}(f) > \epsilon}
\end{align*}
We want to bound the probability of event $A$. Consider the following event $B$:
\begin{align*}
B = \left\{\sup_{f \in \mathcal{F}} |R_{\text{emp}}(f) - R'_{\text{emp}}(f)| > \frac{\epsilon}{2}\right\}
\end{align*}
We will show that $A \subseteq B \cup B'$, where $B'$ is the same event as $B$ but with the roles of $S$ and $S'$ swapped.
Suppose event $A$ occurs, i.e., there exists a function $f \in \mathcal{F}$ such that $R(f) - R_{\text{emp}}(f) > \epsilon$. Then, we have:
\begin{align*}
R(f) - R_{\text{emp}}(f) &> \epsilon \
R(f) - R'{\text{emp}}(f) + R'{\text{emp}}(f) - R_{\text{emp}}(f) &> \epsilon \
\left[R(f) - R'{\text{emp}}(f)\right] + \left[R'{\text{emp}}(f) - R_{\text{emp}}(f)\right] &> \epsilon
\end{align*}
If $R(f) - R'{\text{emp}}(f) \leq \epsilon/2$, then we must have $R'{\text{emp}}(f) - R_{\text{emp}}(f) > \epsilon/2$, which implies event $B$ occurs.
On the other hand, if $R(f) - R'{\text{emp}}(f) > \epsilon/2$, then by swapping the roles of $S$ and $S'$, we have $R'{\text{emp}}(f) - R_{\text{emp}}(f) > \epsilon/2$, which implies event $B'$ occurs.
Therefore, $A \subseteq B \cup B'$, and by the union bound, we have:
\begin{align*}
\mathbb{P}[A] \leq \mathbb{P}[B] + \mathbb{P}[B']
\end{align*}
Since $S$ and $S'$ are drawn independently from the same distribution, we have $\mathbb{P}[B] = \mathbb{P}[B']$. Thus,
\begin{align*}
\mathbb{P}[A] \leq 2\mathbb{P}[B]
\end{align*}
which is equivalent to:
\begin{align*}
\mathbb{P}\left[R(f) - R_{\text{emp}}(f) > \epsilon\right] \leq 2\mathbb{P}\left[\sup_{f \in \mathcal{F}} |R_{\text{emp}}(f) - R'_{\text{emp}}(f)| > \frac{\epsilon}{2}\right]
\end{align*}
This completes the proof.
\end{proof}
% \begin{theorem}[Fairness Generalization Bound]\label{thm:generalization}
% \begin{restatable}[Fairness Generalization Bound]{theorem}{thmgeneralization}\label{thm:generalization}
% Under Assumption \ref{assm:parity}, given the fairness problem as defined in Definition \ref{eqn:def_fairness} with $k$ demographic groups and a function space $\mathcal{F}$ with VC dimension $d_{\text{VC}}(\mathcal{F})$, for any $\delta > 0$, with probability at least $1 - \delta$, for all $f \in \mathcal{F}$:
% \begin{align*}
% \max_{i, j} |R_i(f) - R_j(f)| \leq \max_{i, j} |R_{\text{emp}, i}(f) - R_{\text{emp}, j}(f)| + M\sqrt{\frac{8(d_{\text{VC}}(\mathcal{F})\ln(2em/d_{\text{VC}}(\mathcal{F})) + \ln(4k^2/\delta))}{m}}
% \end{align*}
% where $R_i(f) = \mathbb{E}_{(x, y) \sim \mathcal{D}_{a_i}}[\ell(f(x), y)]$ is the expected risk for group $a_i$, $R_{\text{emp}, i}(f) = \frac{1}{m_i}\sum_{j=1}^{m_i} \ell(f(x_{j}^{(i)}), y_{j}^{(i)})$ is the empirical risk for group $a_i$, $m_i$ is the sample size for group $a_i$, and $m = \sum_{i=1}^k m_i$ is the total sample size.
% \end{restatable}
\thmgeneralization*
\begin{proof}
Let $R(f) = \max_{i, j} |R_i(f) - R_j(f)|$ be the fairness risk and $R_\text{emp}(f) = \max_{i, j} |R_{\text{emp}, i}(f) - R_{\text{emp}, j}(f)|$ be the empirical fairness risk.
% \begin{lemma}[Symmetrization]
% For any function $f \in \mathcal{F}$,
% \begin{align*}
% \mathbb{P}\left[R(f) - R_{\text{emp}}(f) > \epsilon\right] \leq 2\mathbb{P}\left[\sup_{f \in \mathcal{F}} |R_{\text{emp}}(f) - R'{\text{emp}}(f)| > \frac{\epsilon}{2}\right]
% \end{align*}
% where $R'{\text{emp}}(f)$ is the empirical fairness risk on a ghost sample of size $m$ drawn from the same distribution as the original sample.
% \end{lemma}
% The proof of the lemma follows from the same argument as in the symmetrization lemma in the attached file, applied to the fairness risk.
Based on Lemma \ref{thm:symmetrization}, by the VC dimension bound in the attached file, we have:
\begin{align*}
\mathbb{P}\left[\sup_{f \in \mathcal{F}} |R_{\text{emp}}(f) - R'_{\text{emp}}(f)| > \frac{\epsilon}{2}\right] \leq 4\Phi(2m)\exp\left(-\frac{m\epsilon^2}{8M^2}\right)
\end{align*}
where $\Phi(m) = \sum_{i=0}^{d_{\text{VC}}(\mathcal{F})} \binom{m}{i}$ is the growth function of $\mathcal{F}$.
Using the bound $\Phi(m) \leq \left(\frac{em}{d_{\text{VC}}(\mathcal{F})}\right)^{d_{\text{VC}}(\mathcal{F})}$ and setting the right-hand side to $\delta/(2k^2)$, we get:
\begin{align*}
\mathbb{P}\left[\sup_{f \in \mathcal{F}} |R_{\text{emp}}(f) - R'_{\text{emp}}(f)| > \frac{\epsilon}{2}\right] \leq \frac{\delta}{2k^2}
\end{align*}
Applying the union bound over all pairs of demographic groups, we have:
\begin{align*}
\mathbb{P}\left[\exists i, j: R_i(f) - R_j(f) > \epsilon\right] \leq \delta
\end{align*}
provided that:
\begin{align*}
\epsilon = M\sqrt{\frac{8(d_{\text{VC}}(\mathcal{F})\ln(2em/d_{\text{VC}}(\mathcal{F})) + \ln(4k^2/\delta))}{m}}
\end{align*}
Therefore, with probability at least $1 - \delta$, for all $f \in \mathcal{F}$:
\begin{align*}
\max_{i, j} |R_i(f) - R_j(f)| \leq \max_{i, j} |R_{\text{emp}, i}(f) - R_{\text{emp}, j}(f)| + M\sqrt{\frac{8(d_{\text{VC}}(\mathcal{F})\ln(2em/d_{\text{VC}}(\mathcal{F})) + \ln(4k^2/\delta))}{m}}
\end{align*}
This completes the proof.
\end{proof}

% -----------------

% \begin{assumption}[Bounded Loss and Lipschitz Continuity]
% Assume that the loss function $\ell$ is bounded, i.e., $0 \leq \ell(\hat{y}, y) \leq M$ for some constant $M > 0$. Furthermore, assume that the loss function $\ell$ is Lipschitz continuous with respect to its first argument, i.e., there exists a constant $L > 0$ such that $|\ell(\hat{y}_1, y) - \ell(\hat{y}_2, y)| \leq L|\hat{y}_1 - \hat{y}_2|$ for all $\hat{y}_1, \hat{y}_2, y$.
% \end{assumption}

\begin{lemma}[Uniform Convergence of Fairness Risk]\label{thm:convg_fair_risk}
Under Assumption \ref{assm:Lipschitz}, for any $\delta > 0$, with probability at least $1 - \delta$ over the random choice of $S$:
\begin{align*}
\sup_{f \in \mathcal{F}} |R(f) - R_{\text{emp}}(f, S)| \leq \frac{2LM}{\sqrt{m}}\left(\sqrt{2d_{\text{VC}}(\mathcal{F})\ln\frac{em}{d_{\text{VC}}(\mathcal{F})}} + \sqrt{2\ln\frac{4}{\delta}}\right)
\end{align*}
\end{lemma}
% The proof of the lemma follows from the same argument as in the proof of Theorem , using the Lipschitz continuity of the loss function to bound the covering numbers of the function class $\mathcal{G} = {(x, y) \mapsto \ell(f(x), y) : f \in \mathcal{F}}$.
\begin{proof}
Let $\mathcal{G} = {(x, y) \mapsto \ell(f(x), y) : f \in \mathcal{F}}$ be the function class induced by the loss function $\ell$ and the function class $\mathcal{F}$.
% Step 1: Boundedness and Lipschitz continuity of functions in $\mathcal{G}$.
By Assumption \ref{assm:Lipschitz}, the loss function $\ell$ is bounded by $M$ and Lipschitz continuous with constant $L$. For any function $g \in \mathcal{G}$, we have:
\begin{align*}
|g(x, y)| = |\ell(f(x), y)| \leq M
\end{align*}
and for any $(x_1, y_1), (x_2, y_2)$,
\begin{align*}
|g(x_1, y_1) - g(x_2, y_2)| &= |\ell(f(x_1), y_1) - \ell(f(x_2), y_2)| \
&\leq L|f(x_1) - f(x_2)| \
&\leq LD|x_1 - x_2|
\end{align*}
where $D$ is the Lipschitz constant of functions in $\mathcal{F}$. Therefore, functions in $\mathcal{G}$ are bounded by $M$ and Lipschitz continuous with constant $LD$.
% Step 2: Concentration inequality.
By McDiarmid's inequality, for any $f \in \mathcal{F}$, with probability at least $1 - \delta/2$,
\begin{align*}
|R(f) - R_{\text{emp}}(f, S)| \leq M\sqrt{\frac{2\ln(2/\delta)}{m}}
\end{align*}
% Step 3: Covering number bound.
Let $N(\epsilon, \mathcal{F}, |\cdot|\infty)$ be the $\epsilon$-covering number of $\mathcal{F}$ with respect to the $L\infty$ norm. By the Lipschitz continuity of the loss function, we have:
\begin{align*}
N(\epsilon, \mathcal{G}, |\cdot|\infty) \leq N(\epsilon/L, \mathcal{F}, |\cdot|\infty)
\end{align*}
By the VC dimension bound on the covering number \cite{van1997weak},
% (Theorem 2.6.7 in \cite{van1997weak}), 
we have:
\begin{align*}
N(\epsilon/L, \mathcal{F}, |\cdot|\infty) \leq \left(\frac{2eL}{\epsilon}\right)^{d{\text{VC}}(\mathcal{F})}
\end{align*}
% Step 4: Uniform convergence.
By the union bound and the covering number bound, with probability at least $1 - \delta/2$, for all $f \in \mathcal{F}$,
\begin{align*}
|R(f) - R_{\text{emp}}(f, S)| \leq M\sqrt{\frac{2(d_{\text{VC}}(\mathcal{F})\ln(2eL/\epsilon) + \ln(2/\delta))}{m}}
\end{align*}
Setting $\epsilon = LM\sqrt{\frac{2d_{\text{VC}}(\mathcal{F})\ln(em/d_{\text{VC}}(\mathcal{F}))}{m}}$, we get:
\begin{align*}
\sup_{f \in \mathcal{F}} |R(f) - R_{\text{emp}}(f, S)| \leq \frac{2LM}{\sqrt{m}}\left(\sqrt{2d_{\text{VC}}(\mathcal{F})\ln\frac{em}{d_{\text{VC}}(\mathcal{F})}} + \sqrt{2\ln\frac{4}{\delta}}\right)
\end{align*}
with probability at least $1 - \delta$ over the random choice of $S$. This completes the proof.
\end{proof}

% \begin{theorem}[Convergence of Fairness Risk Minimizer]\label{thm:convergence}
% \begin{restatable}[Convergence of Fairness Risk Minimizer]{theorem}{thmconvg}\label{thm:convergence}
% Let $\mathcal{F}$ be a function space with VC dimension $d_{\text{VC}}(\mathcal{F})$ and let $f^* = \arg\min_{f \in \mathcal{F}} R(f)$ be the fairness risk minimizer. Let $\hat{f}_S = \arg\min_{f \in \mathcal{F}} R_{\text{emp}}(f, S)$ be the empirical fairness risk minimizer based on a training set $S$ of size $m$. Then, under Assumption \ref{assm:Lipschitz}, for any $\delta > 0$, with probability at least $1 - \delta$ over the random choice of $S$:
% \begin{align*}
% R(\hat{f}_S) - R(f^*) \leq \frac{2LM}{\sqrt{m}}\left(\sqrt{2d{\text{VC}}(\mathcal{F})\ln\frac{em}{d_{\text{VC}}(\mathcal{F})}} + \sqrt{2\ln\frac{4}{\delta}}\right)
% \end{align*}
% \end{restatable}
\thmconvg*
\begin{proof}
The proof relies on Lemma \ref{thm:convg_fair_risk}.
Let $\epsilon = \frac{2LM}{\sqrt{m}}\left(\sqrt{2d_{\text{VC}}(\mathcal{F})\ln\frac{em}{d_{\text{VC}}(\mathcal{F})}} + \sqrt{2\ln\frac{4}{\delta}}\right)$. By the lemma, with probability at least $1 - \delta$ over the random choice of $S$:
\begin{align*}
R(\hat{f}_S) &\leq R_{\text{emp}}(\hat{f}_S, S) + \epsilon \
&\leq R_{\text{emp}}(f^, S) + \epsilon \
&\leq R(f^) + 2\epsilon
\end{align*}
Therefore, with probability at least $1 - \delta$ over the random choice of $S$:
\begin{align*}
R(\hat{f}_S) - R(f^*) \leq \frac{2LM}{\sqrt{m}}\left(\sqrt{2d{\text{VC}}(\mathcal{F})\ln\frac{em}{d_{\text{VC}}(\mathcal{F})}} + \sqrt{2\ln\frac{4}{\delta}}\right)
\end{align*}
This completes the proof.
\end{proof}

% -----------------

% \begin{assumption}[Bounded Loss and Lipschitz Continuity]
% Assume that the loss function $\ell$ is bounded, i.e., $0 \leq \ell(\hat{y}, y) \leq M$ for some constant $M > 0$. Furthermore, assume that the loss function $\ell$ is Lipschitz continuous with respect to its first argument, i.e., there exists a constant $L > 0$ such that $|\ell(\hat{y}_1, y) - \ell(\hat{y}_2, y)| \leq L|\hat{y}_1 - \hat{y}_2|$ for all $\hat{y}_1, \hat{y}_2, y$.
% \end{assumption}
\begin{lemma}[Risk Bound for Normal Distributions]\label{thm:risk_bound}
Let $p_i$ and $p$ be the density functions of two normal distributions with means $\mu_i$ and $\mu$, and covariance matrices $\Sigma_i$ and $\Sigma$, respectively. Then, for any function $f$:
\begin{align*}
\left|\mathbb{E}_{(x, y) \sim p_i}[f(x, y)] - \mathbb{E}_{(x, y) \sim p}[f(x, y)]\right| \leq L_f|\mu_i - \mu|_2 + L_f\sqrt{|\Sigma_i - \Sigma|_F}
\end{align*}
where $L_f$ is the Lipschitz constant of $f$ with respect to the Euclidean norm.
\end{lemma}
\begin{proof}
Let $\mathcal{P}(\mathbb{R}^d \times \mathbb{R})$ be the set of all probability measures on $\mathbb{R}^d \times \mathbb{R}$, and let $\Pi(p_i, p)$ be the set of all joint probability measures on $(\mathbb{R}^d \times \mathbb{R}) \times (\mathbb{R}^d \times \mathbb{R})$ with marginals $p_i$ and $p$.
The Kantorovich-Rubinstein duality states that for any Lipschitz function $f$ with Lipschitz constant $L_f$, we have:
\begin{align}
\left|\mathbb{E}{(x, y) \sim p_i}[f(x, y)] - \mathbb{E}{(x, y) \sim p}[f(x, y)]\right| \leq L_f \cdot W_1(p_i, p) \label{eq:KR_duality}
\end{align}
where $W_1(p_i, p)$ is the 1-Wasserstein distance between $p_i$ and $p$, defined as:
\begin{align}
W_1(p_i, p) = \inf_{\gamma \in \Pi(p_i, p)} \mathbb{E}_{((x, y), (x', y')) \sim \gamma}[|(x, y) - (x', y')|_2] \label{eq:W1_distance}
\end{align}
Now, let's focus on bounding the 1-Wasserstein distance between two normal distributions $p_i = \mathcal{N}(\mu_i, \Sigma_i)$ and $p = \mathcal{N}(\mu, \Sigma)$. By the triangular inequality, we have:
\begin{align}
W_1(p_i, p) &\leq \inf_{\gamma \in \Pi(p_i, p)} \mathbb{E}{((x, y), (x', y')) \sim \gamma}[|x - x'|2] + \inf{\gamma \in \Pi(p_i, p)} \mathbb{E}{((x, y), (x', y')) \sim \gamma}[|y - y'|_2] \label{eq:W1_bound_1} \\
&\leq W_1(\mathcal{N}(\mu_i, \Sigma_i), \mathcal{N}(\mu, \Sigma_i)) + W_1(\mathcal{N}(\mu, \Sigma_i), \mathcal{N}(\mu, \Sigma)) \label{eq:W1_bound_2}
\end{align}
The first term in \eqref{eq:W1_bound_2} can be bounded by the mean difference:
\begin{align}
W_1(\mathcal{N}(\mu_i, \Sigma_i), \mathcal{N}(\mu, \Sigma_i)) \leq |\mu_i - \mu|_2 \label{eq:W1_bound_mean}
\end{align}
The second term in \eqref{eq:W1_bound_2} can be bounded by the covariance difference \cite{givens1984class}:
\begin{align}
W_1(\mathcal{N}(\mu, \Sigma_i), \mathcal{N}(\mu, \Sigma)) \leq \sqrt{|\Sigma_i - \Sigma|_F} \label{eq:W1_bound_cov}
\end{align}
Combining \eqref{eq:KR_duality}, \eqref{eq:W1_bound_2}, \eqref{eq:W1_bound_mean}, and \eqref{eq:W1_bound_cov}, we obtain:
\begin{align*}
\left|\mathbb{E}{(x, y) \sim p_i}[f(x, y)] - \mathbb{E}{(x, y) \sim p}[f(x, y)]\right| \leq L_f|\mu_i - \mu|_2 + L_f\sqrt{|\Sigma_i - \Sigma|_F}
\end{align*}
which completes the proof.
\end{proof}
% \begin{theorem}[Group-Specific Risk Bound Theorem for Normal Distributions]\label{thm:group_risk}
% \begin{restatable}[Group-Specific Risk Bound Theorem for Normal Distributions]{theorem}{thmgrouprisk}\label{thm:group_risk}
% Let $\mathcal{F}$ be a function space with VC dimension $d_{\text{VC}}(\mathcal{F})$ and let $f^*_i = \arg\min_{f \in \mathcal{F}} R_i(f)$ be the risk minimizer for demographic group $a_i$. Let $\hat{f}_S = \arg\min_{f \in \mathcal{F}} R_{\text{emp}}(f, S)$ be the empirical risk minimizer based on a training set $S$ of size $m$ drawn from the overall data distribution. Then, under Assumptions \ref{assm:Lipschitz} and \ref{assm:distribution}, for any $\delta > 0$, with probability at least $1 - \delta$ over the random choice of $S$:
% \begin{align*}
% R_i(\hat{f}_S) - R_i(f^*_i) \leq \frac{2LM}{\sqrt{m}}\left(\sqrt{2d{\text{VC}}(\mathcal{F})\ln\frac{em}{d{\text{VC}}(\mathcal{F})}} + \sqrt{2\ln\frac{4}{\delta}}\right) + L|\mu_i - \mu|2 + L\sqrt{|\Sigma_i - \Sigma|F}
% \end{align*}
% where $R_i(f) = \mathbb{E}_{(x, y) \sim \mathcal{D}_{a_i}}[\ell(f(x), y)]$ is the expected risk for group $a_i$, $R_{\text{emp}}(f, S) = \frac{1}{m}\sum_{j=1}^m \ell(f(x_j), y_j)$ is the empirical risk based on the training set $S$, $\mu$ and $\Sigma$ are the mean and covariance matrix of the overall data distribution, and $|\cdot|_F$ denotes the Frobenius norm.
% \end{restatable}
\thmgrouprisk*
\begin{proof}
The proof relies on Lemma \ref{thm:risk_bound}.
% \begin{lemma}[Risk Bound for Normal Distributions]\label{thm:risk_bound}
% Let $p_i$ and $p$ be the density functions of two normal distributions with means $\mu_i$ and $\mu$, and covariance matrices $\Sigma_i$ and $\Sigma$, respectively. Then, for any function $f$:
% \begin{align*}
% \left|\mathbb{E}_{(x, y) \sim p_i}[f(x, y)] - \mathbb{E}_{(x, y) \sim p}[f(x, y)]\right| \leq L_f|\mu_i - \mu|_2 + L_f\sqrt{|\Sigma_i - \Sigma|_F}
% \end{align*}
% where $L_f$ is the Lipschitz constant of $f$ with respect to the Euclidean norm.
% \end{lemma}
% The proof of the lemma follows from the Kantorovich-Rubinstein duality and the fact that the Wasserstein distance between two normal distributions can be bounded by their mean and covariance differences.
Let $\epsilon = \frac{2LM}{\sqrt{m}}\left(\sqrt{2d_{\text{VC}}(\mathcal{F})\ln\frac{em}{d_{\text{VC}}(\mathcal{F})}} + \sqrt{2\ln\frac{4}{\delta}}\right)$. By Lemma \ref{thm:convg_fair_risk}, with probability at least $1 - \delta$ over the random choice of $S$::
\begin{align*}
R_{\text{emp}}(\hat{f}_S, S) - R(\hat{f}_S) \leq \epsilon, \hspace{2ex}
R_{\text{emp}}(f^*_i, S) - R(f^*_i) \geq -\epsilon
\end{align*}
Applying Lemma \ref{thm:risk_bound} with $f(x, y) = \ell(\hat{y}, y)$, which has Lipschitz constant $L$ by Assumption \ref{assm:Lipschitz}, we have:
\begin{align*}
R_i(f) - R(f) &\leq L|\mu_i - \mu|_2 + L\sqrt{|\Sigma_i - \Sigma|_F}, \quad \forall f \in \mathcal{F}
\end{align*}
Combining the above inequalities, with probability at least $1 - \delta$ over the random choice of $S$:
\begin{align*}
R_i(\hat{f}_S) - R_i(f^*_i) &= R_i(\hat{f}_S) - R(\hat{f}_S) + R(\hat{f}_S) - R_{\text{emp}}(\hat{f}_S, S) \\
&\quad + R_{\text{emp}}(\hat{f}_S, S) - R_{\text{emp}}(f^*_i, S) + R_{\text{emp}}(f^*_i, S) - R(f^*_i) \\
&\quad + R(f^*_i) - R_i(f^*_i) \\
&\leq L|\mu_i - \mu|_2 + L\sqrt{|\Sigma_i - \Sigma|_F} + \epsilon + 0 + \epsilon \\
&\quad + L|\mu_i - \mu|2 + L\sqrt{|\Sigma_i - \Sigma|F} \\
&= \frac{2LM}{\sqrt{m}}\left(\sqrt{2d{\text{VC}}(\mathcal{F})\ln\frac{em}{d{\text{VC}}(\mathcal{F})}} + \sqrt{2\ln\frac{4}{\delta}}\right) \\
&\quad + 2L|\mu_i - \mu|_2 + 2L\sqrt{|\Sigma_i - \Sigma|_F}
\end{align*}
This completes the proof.
\end{proof}

% \begin{theorem}[Expected Loss Bound for Demographic Group with Normal Distribution]\label{thm:accuracy}
% \begin{restatable}[Expected Loss Bound for Demographic Group with Normal Distribution]{theorem}{thmaccuracy}\label{thm:accuracy}
% Let $\mathcal{D}_{a_i} \sim \mathcal{N}(\mu_i, \Sigma_i)$ be the data distribution for demographic group $a_i$, and let $\mathcal{D} \sim \mathcal{N}(\mu, \Sigma)$ be the overall data distribution. Let $f(\cdot)$ be a function that maps input $x$ to predicted labels $\hat{y}$, and let $\ell$ be a loss function bounded by $B$, i.e., $|\ell(f(x), y)| \leq B$ for all $x, y$. Suppose we have a training set ${(x_j, y_j)}_{j=1}^n$ of size $n$ drawn independently from $\mathcal{D}$. Then, with probability at least $1-\delta$, the expected loss of $f(\cdot)$ on $\mathcal{D}_{a_i}$ is bounded as follows:
% \begin{align*}
% \mathbb{E}_{(x, y) \sim \mathcal{D}_{a_i}}[\ell(f(x), y)] \leq \mathbb{E}_{(x, y) \sim \mathcal{D}}[\ell(f(x), y)] + B|\mu_i - \mu|_2 + B\sqrt{|\Sigma_i - \Sigma|_F}
% \end{align*}
% \end{restatable}
\thmaccuracy*
\begin{proof}
We start by applying the reference theorem to the overall data distribution $\mathcal{D}$:
\begin{align*}
\mathbb{E}_{(x, y) \sim \mathcal{D}}[\ell(f(x), y)] \leq \frac{1}{n}\sum_{j=1}^n \ell(f(x_j), y_j) + B\sqrt{\frac{2|\Sigma|\log(2/\delta)}{n}}
\end{align*}
Now, we use Lemma \ref{thm:risk_bound} to relate the expected loss on $\mathcal{D}_{a_i}$ to the expected loss on $\mathcal{D}$:
% \begin{lemma}[Risk Bound for Normal Distributions]\label{thm:risk_bound_distribution}
% Let $p_i$ and $p$ be the density functions of two normal distributions with means $\mu_i$ and $\mu$, and covariance matrices $\Sigma_i$ and $\Sigma$, respectively. Then, for any function $f$:
% \begin{align*}
% \left|\mathbb{E}_{(x, y) \sim p_i}[f(x, y)] - \mathbb{E}_{(x, y) \sim p}[f(x, y)]\right| \leq L_f|\mu_i - \mu|_2 + L_f\sqrt{|\Sigma_i - \Sigma|_F}
% \end{align*}
% where $L_f$ is the Lipschitz constant of $f$ with respect to the Euclidean norm.
% \end{lemma}
% The proof of the lemma follows from the Kantorovich-Rubinstein duality and the fact that the Wasserstein distance between two normal distributions can be bounded by their mean and covariance differences.
Applying the lemma with $f(x, y) = \ell(f(x), y)$, which has Lipschitz constant $B$ since $\ell$ is bounded by $B$, we have:
\begin{align*}
\left|\mathbb{E}_{(x, y) \sim \mathcal{D}_{a_i}}[\ell(f(x), y)] - \mathbb{E}_{(x, y) \sim \mathcal{D}}[\ell(f(x), y)]\right| \leq B|\mu_i - \mu|_2 + B\sqrt{|\Sigma_i - \Sigma|_F}
\end{align*}
Rearranging the terms, we get:
\begin{align*}
\mathbb{E}_{(x, y) \sim \mathcal{D}_{a_i}}[\ell(f(x), y)] \leq \mathbb{E}_{(x, y) \sim \mathcal{D}}[\ell(f(x), y)] + B|\mu_i - \mu|_2 + B\sqrt{|\Sigma_i - \Sigma|_F}
\end{align*}
This completes the proof.
\end{proof}

% \begin{corollary}[Fairness-Accuracy Trade-off]\label{thm:fairness_accuracy}
% \begin{restatable}[Expected Loss Bound for Demographic Group with Normal Distribution]{theorem}{thmaccuracy}\label{thm:accuracy}
% Let $\mathcal{F}$ be a function space with VC dimension $d_{VC}(\mathcal{F})$, and let $f^* = \arg\min_{f \in \mathcal{F}} R(f)$ and $f_i^* = \arg\min_{f \in \mathcal{F}} R_i(f)$ be the fairness and accuracy risk minimizers, respectively. Let $\hat{f}_S = \arg\min_{f \in \mathcal{F}} R_{emp}(f, S)$ be the empirical fairness risk minimizer based on a training set $S$ of size $m$ drawn from the overall data distribution. Then, under Assumptions \ref{assm:prevalence}, \ref{assm:Lipschitz}, and \ref{assm:distribution}, for any $\delta > 0$, with probability at least $1 - \delta$ over the random choice of $S$:
% \begin{align*}
% R_i(f^*) - R_i(f_i^*) \leq \frac{4LM}{\sqrt{m}} \sqrt{2d_{VC}(\mathcal{F}) \ln \frac{em}{d_{VC}(\mathcal{F})} + 2 \ln \frac{4}{\delta}} + L|\mu_i - \mu|_2 + L\sqrt{|\Sigma_i - \Sigma|_F}
% \end{align*}
% \end{restatable}
\thmaccuracy*
\begin{proof}
By the triangle inequality and Theorems \ref{thm:convergence} and \ref{thm:group_risk}, we have:
\begin{align*}
R_i(f^*) - R_i(f_i^*) &\leq R_i(f^*) - R_i(\hat{f}_S) + R_i(\hat{f}_S) - R_i(f_i^*) \\
&\leq \frac{2LM}{\sqrt{m}} \sqrt{2d_{VC}(\mathcal{F}) \ln \frac{em}{d_{VC}(\mathcal{F})} + 2 \ln \frac{4}{\delta}} \\
&\quad + \frac{2LM}{\sqrt{m}} \sqrt{2d_{VC}(\mathcal{F}) \ln \frac{em}{d_{VC}(\mathcal{F})} + 2 \ln \frac{4}{\delta}} + L|\mu_i - \mu|2 + L\sqrt{|\Sigma_i - \Sigma|F} \\
&= \frac{4LM}{\sqrt{m}} \sqrt{2d{VC}(\mathcal{F}) \ln \frac{em}{d{VC}(\mathcal{F})} + 2 \ln \frac{4}{\delta}} + L|\mu_i - \mu|_2 + L\sqrt{|\Sigma_i - \Sigma|_F}
\end{align*}
This completes the proof.
\end{proof}

% \begin{corollary}[Correlation between Expected Loss Bound and Feature Distance]\label{thm:correlation_lossbound_featdist}
% \begin{restatable}[Correlation between Expected Loss Bound and Feature Distance]{corollary}{thmcorrelationloss}\label{thm:correlation_lossbound_featdist}
% Let $\mathcal{D}_{a_i} \sim \mathcal{N}(\mu_i, \Sigma_i)$ be the data distribution for demographic group $a_i$, and let $\mathcal{D} \sim \mathcal{N}(\mu, \Sigma)$ be the overall data distribution. Let $f(\cdot)$ be a function that maps input $x$ to a discriminative feature $z$ in a metric space, and let $\ell$ be a loss function bounded by $B$, i.e., $|\ell(z, y)| \leq B$ for all $z, y$. Suppose we have a training set ${(x_j, y_j)}{j=1}^n$ of size $n$ drawn independently from $\mathcal{D}$. Let $\bar{z}$ be the centroid of the features generated by $f$ on the overall data distribution, and let $\bar{z}_i$ be the centroid of the features generated by $f$ on the demographic group $a_i$. Then, with probability at least $1-\delta$, the expected loss of $f(\cdot)$ on $\mathcal{D}_{a_i}$ is bounded as follows:
% \begin{align*}
% \mathbb{E}_{(x, y) \sim \mathcal{D}_{a_i}}[\ell(f(x), y)] \leq \mathbb{E}_{(x, y) \sim \mathcal{D}}[\ell(f(x), y)] + B\cdot d(\bar{z}_i, \bar{z}) + B\sqrt{\mathbb{E}_{z \sim f(\mathcal{D}_{a_i})}[d^2(z, \bar{z}_i)] - \mathbb{E}_{z \sim f(\mathcal{D})}[d^2(z, \bar{z})]}
% \end{align*}
% where $d(\cdot, \cdot)$ is a distance function in the metric space.
% \end{restatable}
\thmcorrelationloss*
\begin{proof}
We start by applying Theorem \ref{thm:accuracy} to the discriminative feature space:
\begin{align*}
\mathbb{E}_{(x, y) \sim \mathcal{D}_{a_i}}[\ell(f(x), y)] \leq \mathbb{E}_{(x, y) \sim \mathcal{D}}[\ell(f(x), y)] + B|\mu{z_i} - \mu_z|2 + B\sqrt{|\Sigma{z_i} - \Sigma_z|F}
\end{align*}
where $\mu{z_i}$ and $\Sigma_{z_i}$ are the mean and covariance matrix of the features generated by $f$ on $\mathcal{D}_{a_i}$, and $\mu_z$ and $\Sigma_z$ are the mean and covariance matrix of the features generated by $f$ on $\mathcal{D}$.
By the definition of the centroid, we have $\bar{z}_i = \mu{z_i}$ and $\bar{z} = \mu_z$. Therefore, $|\mu_{z_i} - \mu_z|_2 = d(\bar{z}_i, \bar{z})$.
Now, let's focus on the term $|\Sigma_{z_i} - \Sigma_z|_F$. By the properties of the Frobenius norm and the trace operator \cite{zhang2011matrix}, we have:
\begin{align*}
|\Sigma_{z_i} - \Sigma_z|F &= \sqrt{\text{tr}((\Sigma{z_i} - \Sigma_z)^T(\Sigma_{z_i} - \Sigma_z))} \\
&= \sqrt{\text{tr}(\Sigma_{z_i}^2) - 2\text{tr}(\Sigma_{z_i}\Sigma_z) + \text{tr}(\Sigma_z^2)} \\
&= \sqrt{\mathbb{E}_{z \sim f(\mathcal{D}_{a_i})}[d^2(z, \bar{z}_i)] - 2\mathbb{E}_{z \sim f(\mathcal{D}_{a_i}), z' \sim f(\mathcal{D})}[d(z, z')] + \mathbb{E}_{z \sim f(\mathcal{D})}[d^2(z, \bar{z})]}
\end{align*}
Using the Cauchy-Schwarz inequality, we can bound the cross-term as follows:
\begin{align*}
\mathbb{E}_{z \sim f(\mathcal{D}_{a_i}), z' \sim f(\mathcal{D})}[d(z, z')] &\leq \sqrt{\mathbb{E}_{z \sim f(\mathcal{D}_{a_i})}[d^2(z, \bar{z}_i)] \cdot \mathbb{E}_{z \sim f(\mathcal{D})}[d^2(z, \bar{z})]} \\
&\leq \frac{1}{2}\left(\mathbb{E}_{z \sim f(\mathcal{D}_{a_i})}[d^2(z, \bar{z}_i)] + \mathbb{E}_{z \sim f(\mathcal{D})}[d^2(z, \bar{z})]\right)
\end{align*}
Substituting this bound into the expression for $|\Sigma_{z_i} - \Sigma_z|_F$, we get:
\begin{align*}
|\Sigma_{z_i} - \Sigma_z|F &\leq \sqrt{\mathbb{E}_{z \sim f(\mathcal{D}_{a_i})}[d^2(z, \bar{z}_i)] - \mathbb{E}_{z \sim f(\mathcal{D})}[d^2(z, \bar{z})]}
\end{align*}
Combining the results for $|\mu_{z_i} - \mu_z|2$ and $|\Sigma{z_i} - \Sigma_z|_F$, we obtain the desired bound:
\begin{align*}
\mathbb{E}_{(x, y) \sim \mathcal{D}_{a_i}}[\ell(f(x), y)] \leq \mathbb{E}_{(x, y) \sim \mathcal{D}}[\ell(f(x), y)] + B\cdot d(\bar{z}_i, \bar{z}) + B\sqrt{\mathbb{E}_{z \sim f(\mathcal{D}_{a_i})}[d^2(z, \bar{z}_i)] - \mathbb{E}_{z \sim f(\mathcal{D})}[d^2(z, \bar{z})]}
\end{align*}
This completes the proof.
\end{proof}

\setcounter{figure}{0}  

\subsection{Results on HAM10000}

Figure~\ref{fig_ham} shows the feature distribution, AUC, and Brier Score with EfficientNet for Basal Cell Carcinoma (BCC) detection on the HAM10000 dataset across three attributes: Gender and Age. It can be observed that the overall feature distribution has a mean of 12.39 and a standard deviation of 4.14. For the female group, the mean is 12.25 with a standard deviation of 4.09, while for the male group, the mean is 12.52 with a standard deviation of 4.17. By comparison, it can be found that groups with feature distributions deviating more from the overall distribution tend to have lower AUC values, which aligns with the predictions of Theorem 7 and Corollary 2.

\begin{figure}[h]
    \centering
    \begin{subfigure}{0.5\textwidth}
        \centering
        \includegraphics[width=1.\textwidth]{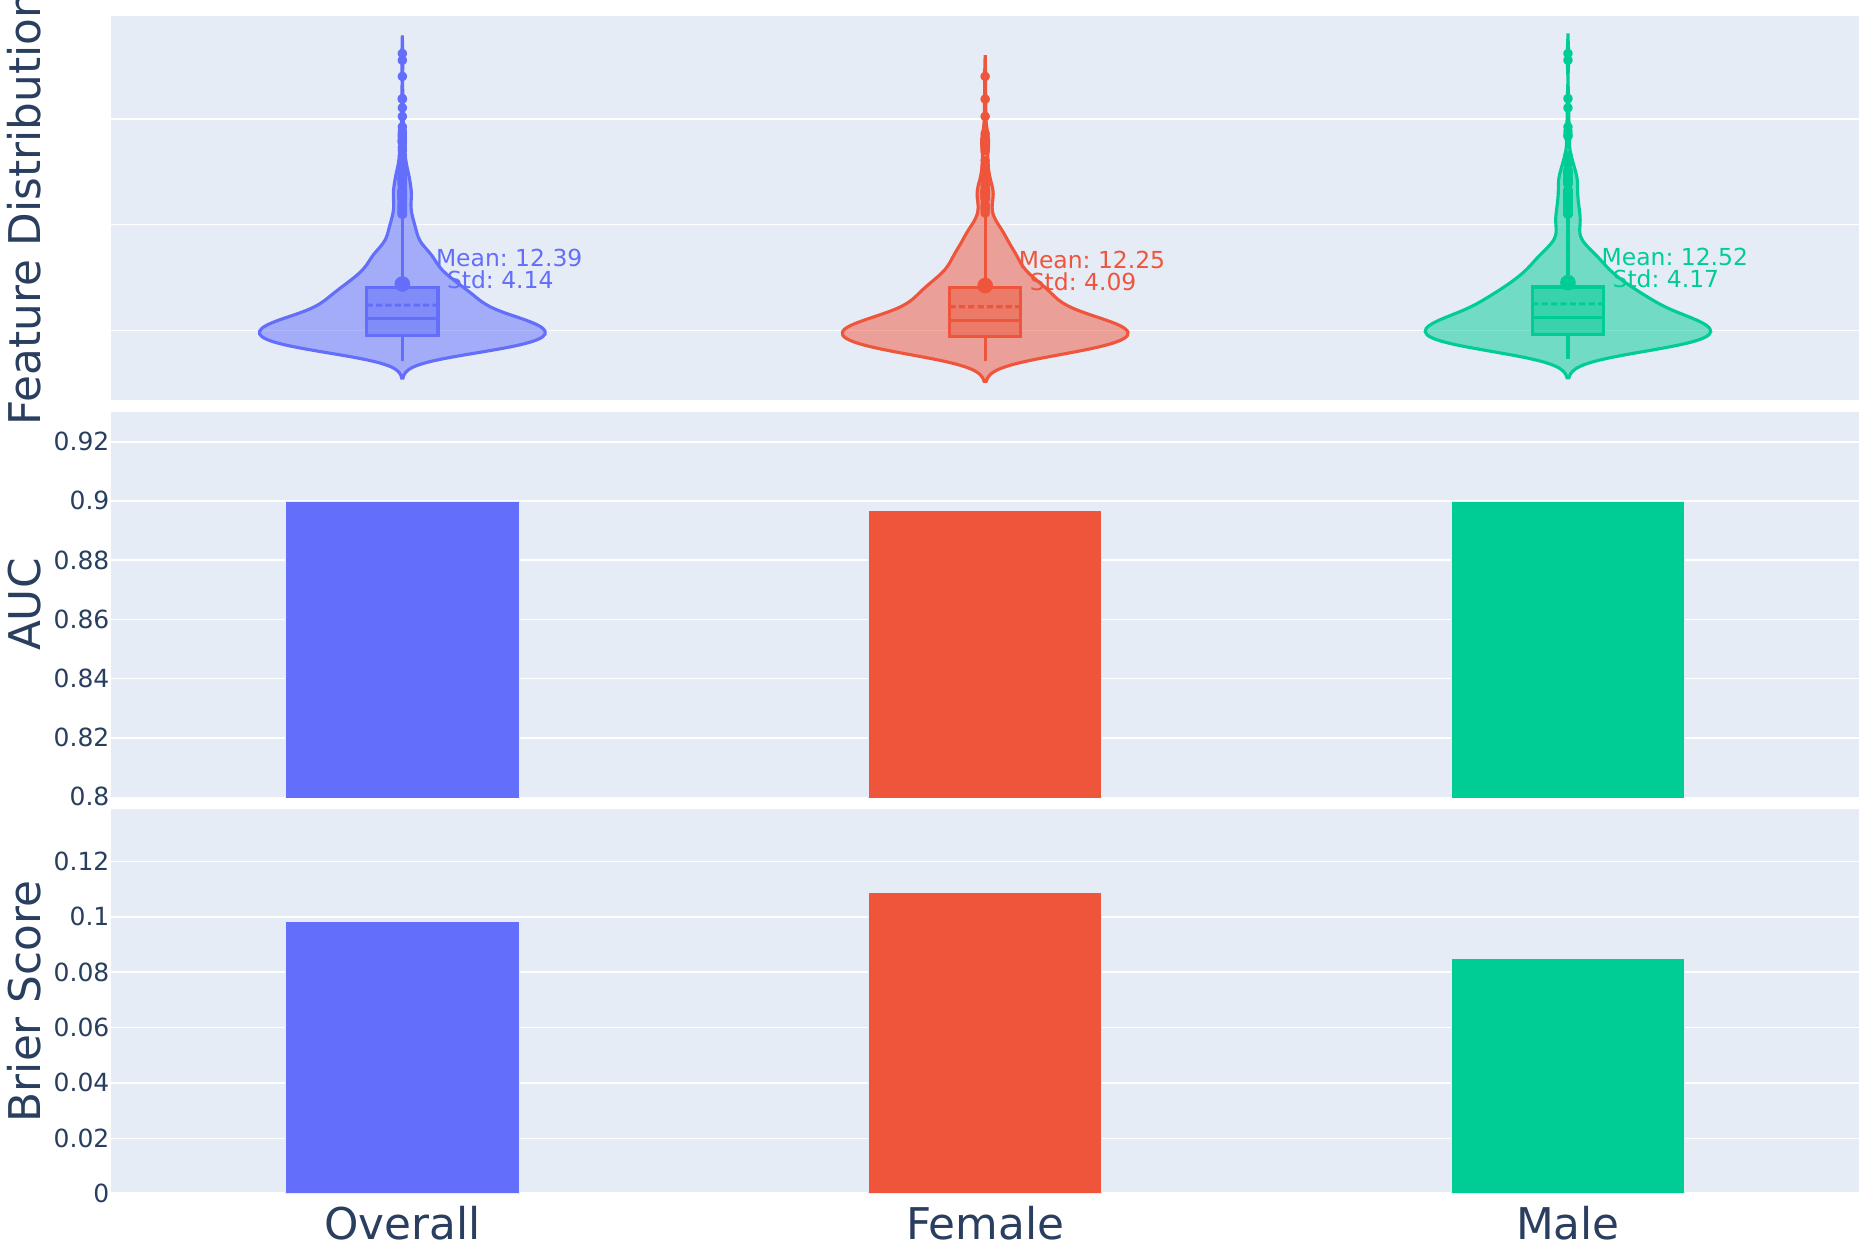}
        \caption{BCC Detection on Gender}
        \label{fig:combination_dr_vit}
    \end{subfigure}%
    \begin{subfigure}{0.5\textwidth}
        \centering
        \includegraphics[width=1.\textwidth]{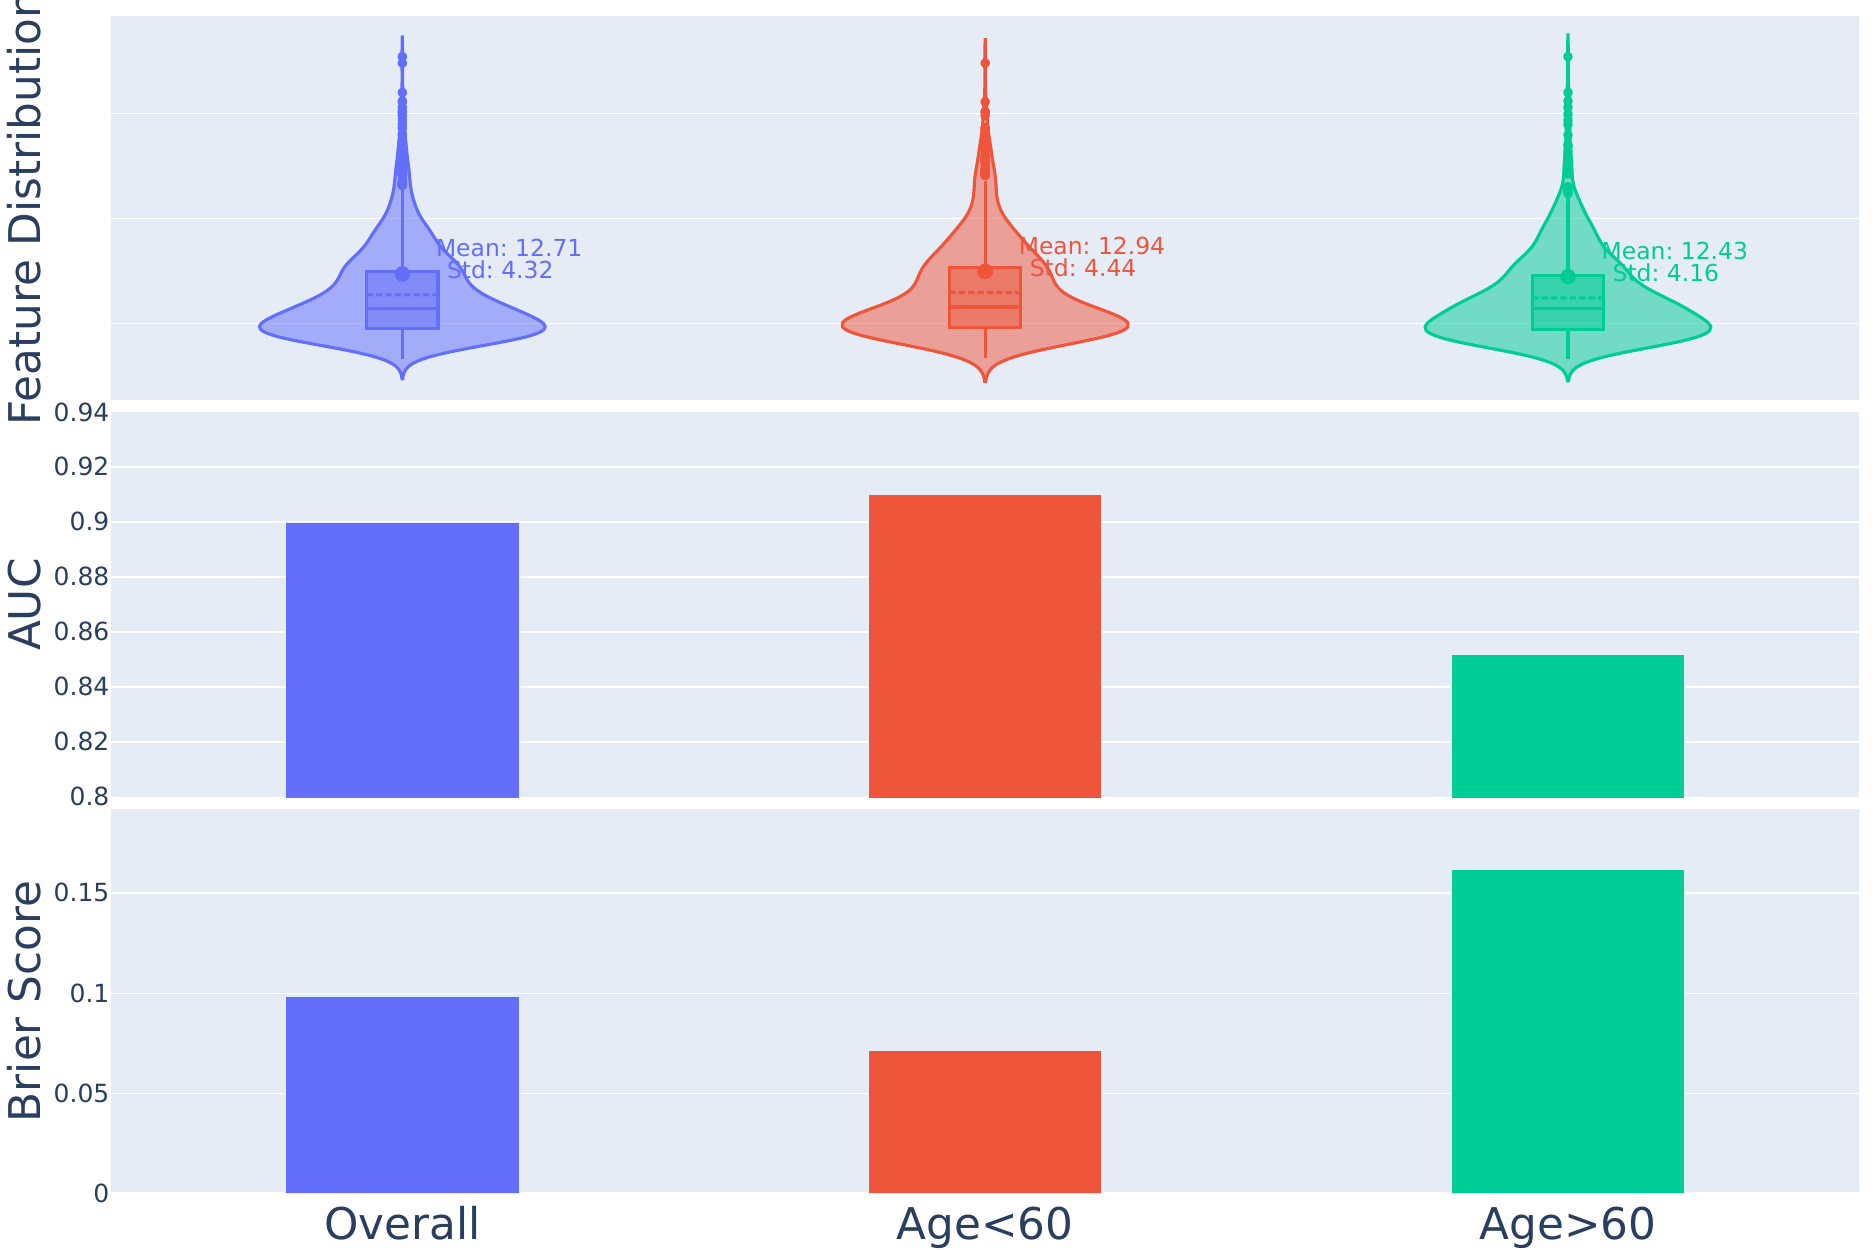}
        \caption{BCC Detection on Age}
        \label{fig:combination_pe_vit}
    \end{subfigure} \\
    \caption{Combination of feature distribution, AUC, and Brier Score with EfficientNet for Basal Cell Carcinoma (BCC) detection on the \textbf{HAM10000 dataset} across two attributes: Gender and Age.}
    \label{fig_ham}
\end{figure}

\subsection{Results on FairFace}

Figure~\ref{fig_fairface} illustrates the feature distribution, AUC, and Brier Score of EfficientNet for glasses detection using the FairFace dataset, evaluated across three different attributes: Age, Skin Color, and Gender. Taking the age group analysis as an example, the overall feature distribution exhibits a mean of 10.21 and a standard deviation of 2.45. Specifically, for the age<35 group, the mean is 9.88 with a standard deviation of 1.87; for the 35<age<65 group, the mean is 10.31 with a standard deviation of 2.56; and for the age>65 group, the mean is 10.29 with a standard deviation of 2.74. A comparative evaluation shows that demographic groups whose feature distributions deviate more significantly from the overall distribution tend to achieve lower AUC values. This observation is in line with the theoretical predictions derived from Theorem 7 and Corollary 2.

\begin{figure}[h]
    \centering
    \begin{subfigure}{0.33\textwidth}
        \centering
        \includegraphics[width=1.\textwidth]{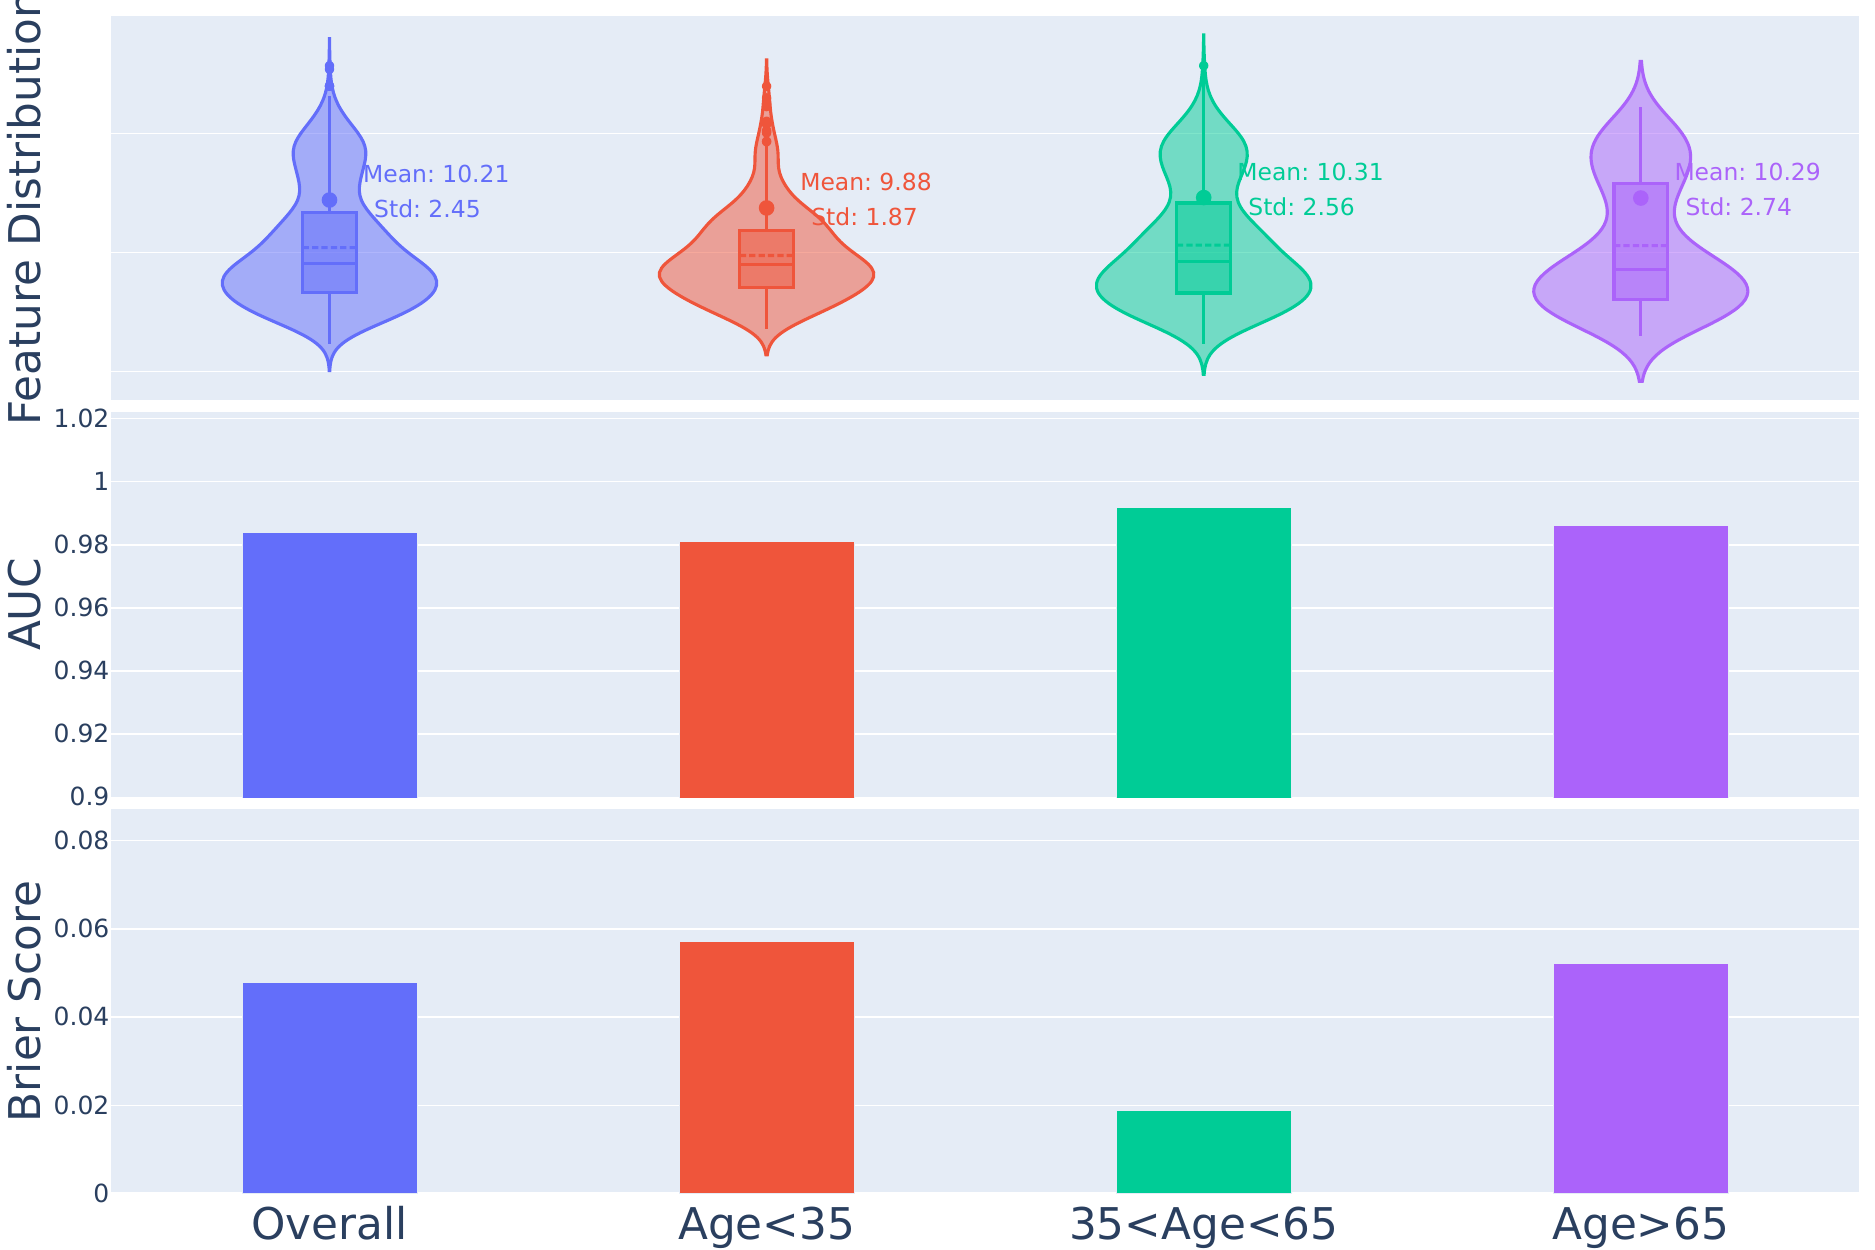}
        \caption{Glasses Detection on Age}
        \label{fig:combination_dr_vit}
    \end{subfigure}%
    \begin{subfigure}{0.33\textwidth}
        \centering
        \includegraphics[width=1.\textwidth]{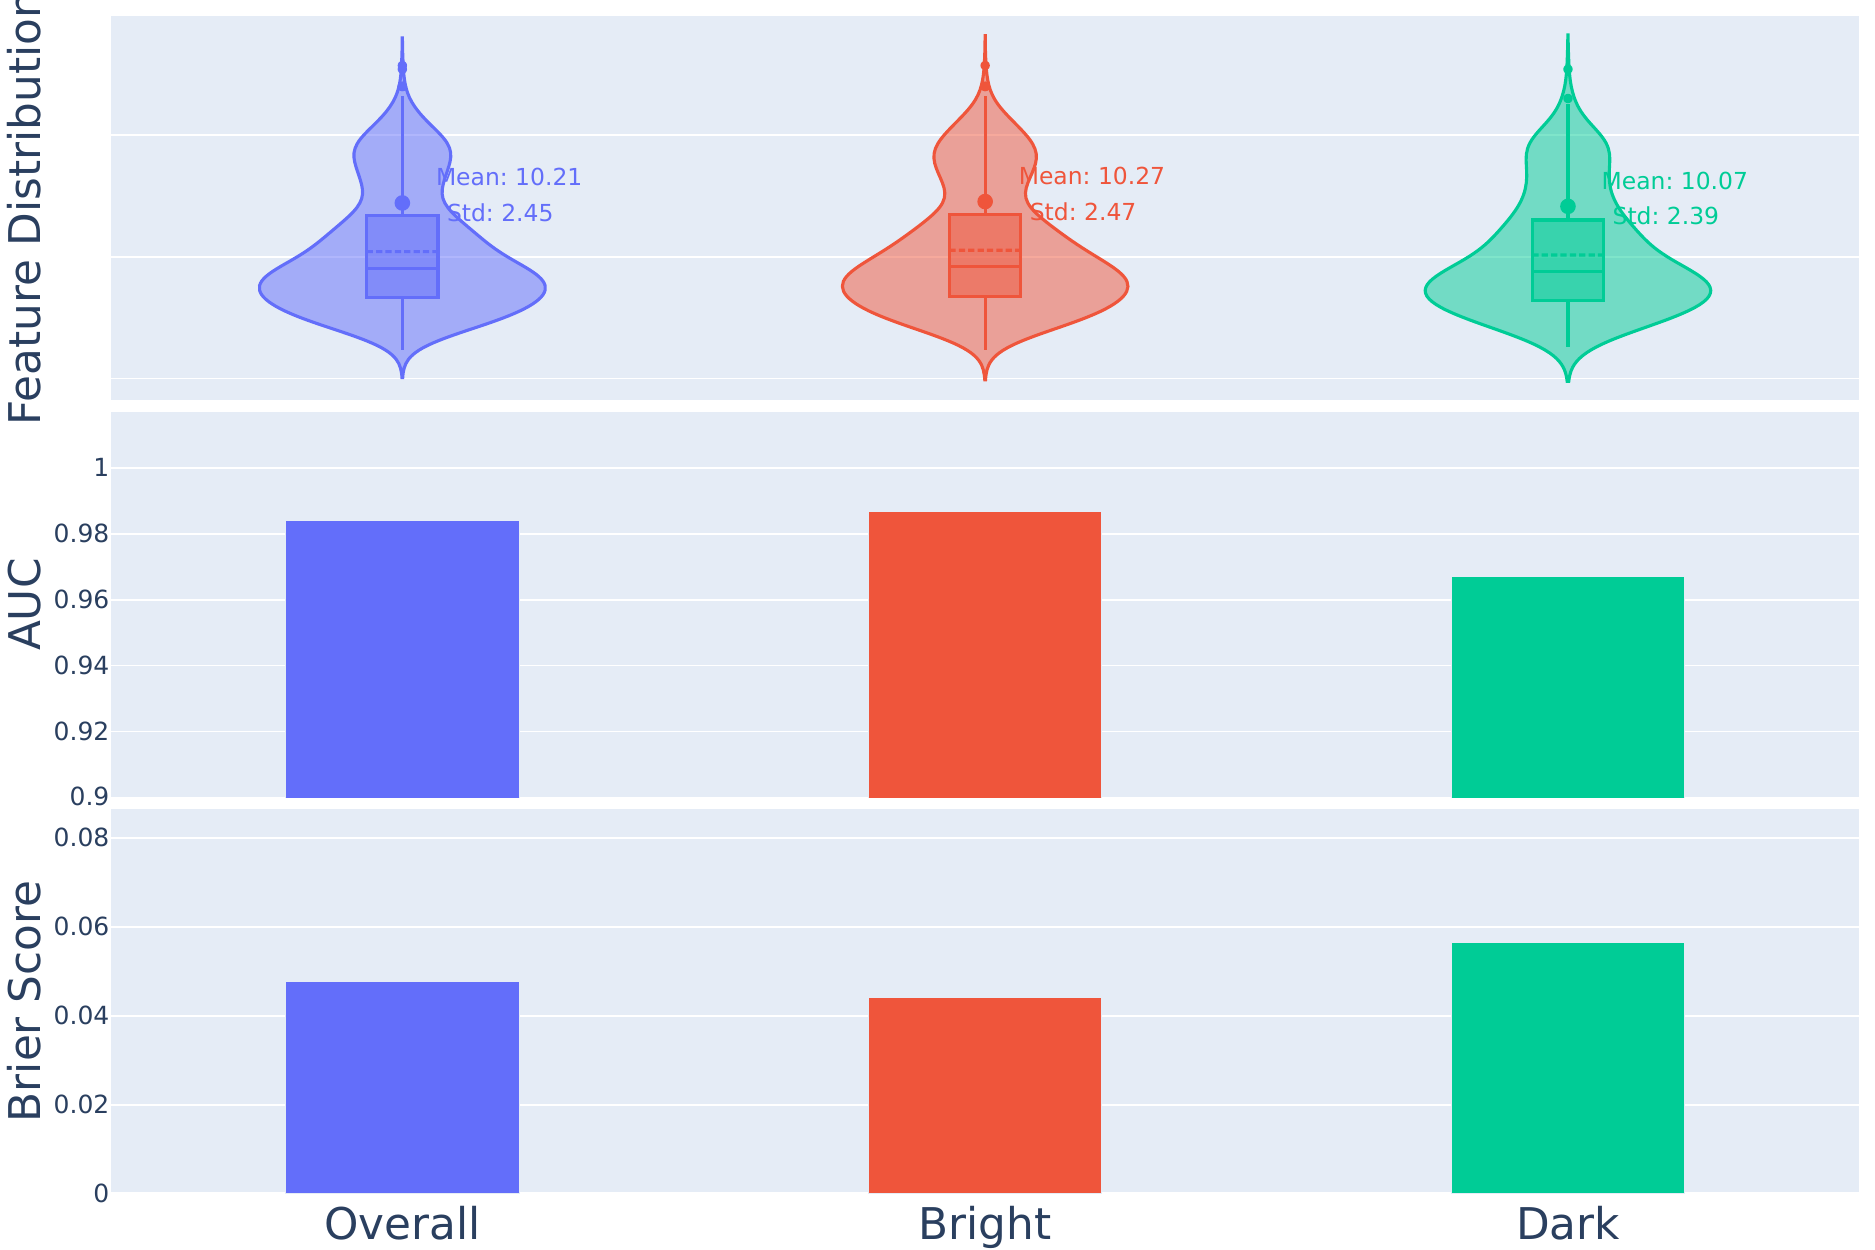}
        \caption{Glasses Detection on Skin Color}
        \label{fig:combination_glaucoma_vit}
    \end{subfigure} 
    \begin{subfigure}{0.33\textwidth}
        \centering
        \includegraphics[width=1.\textwidth]{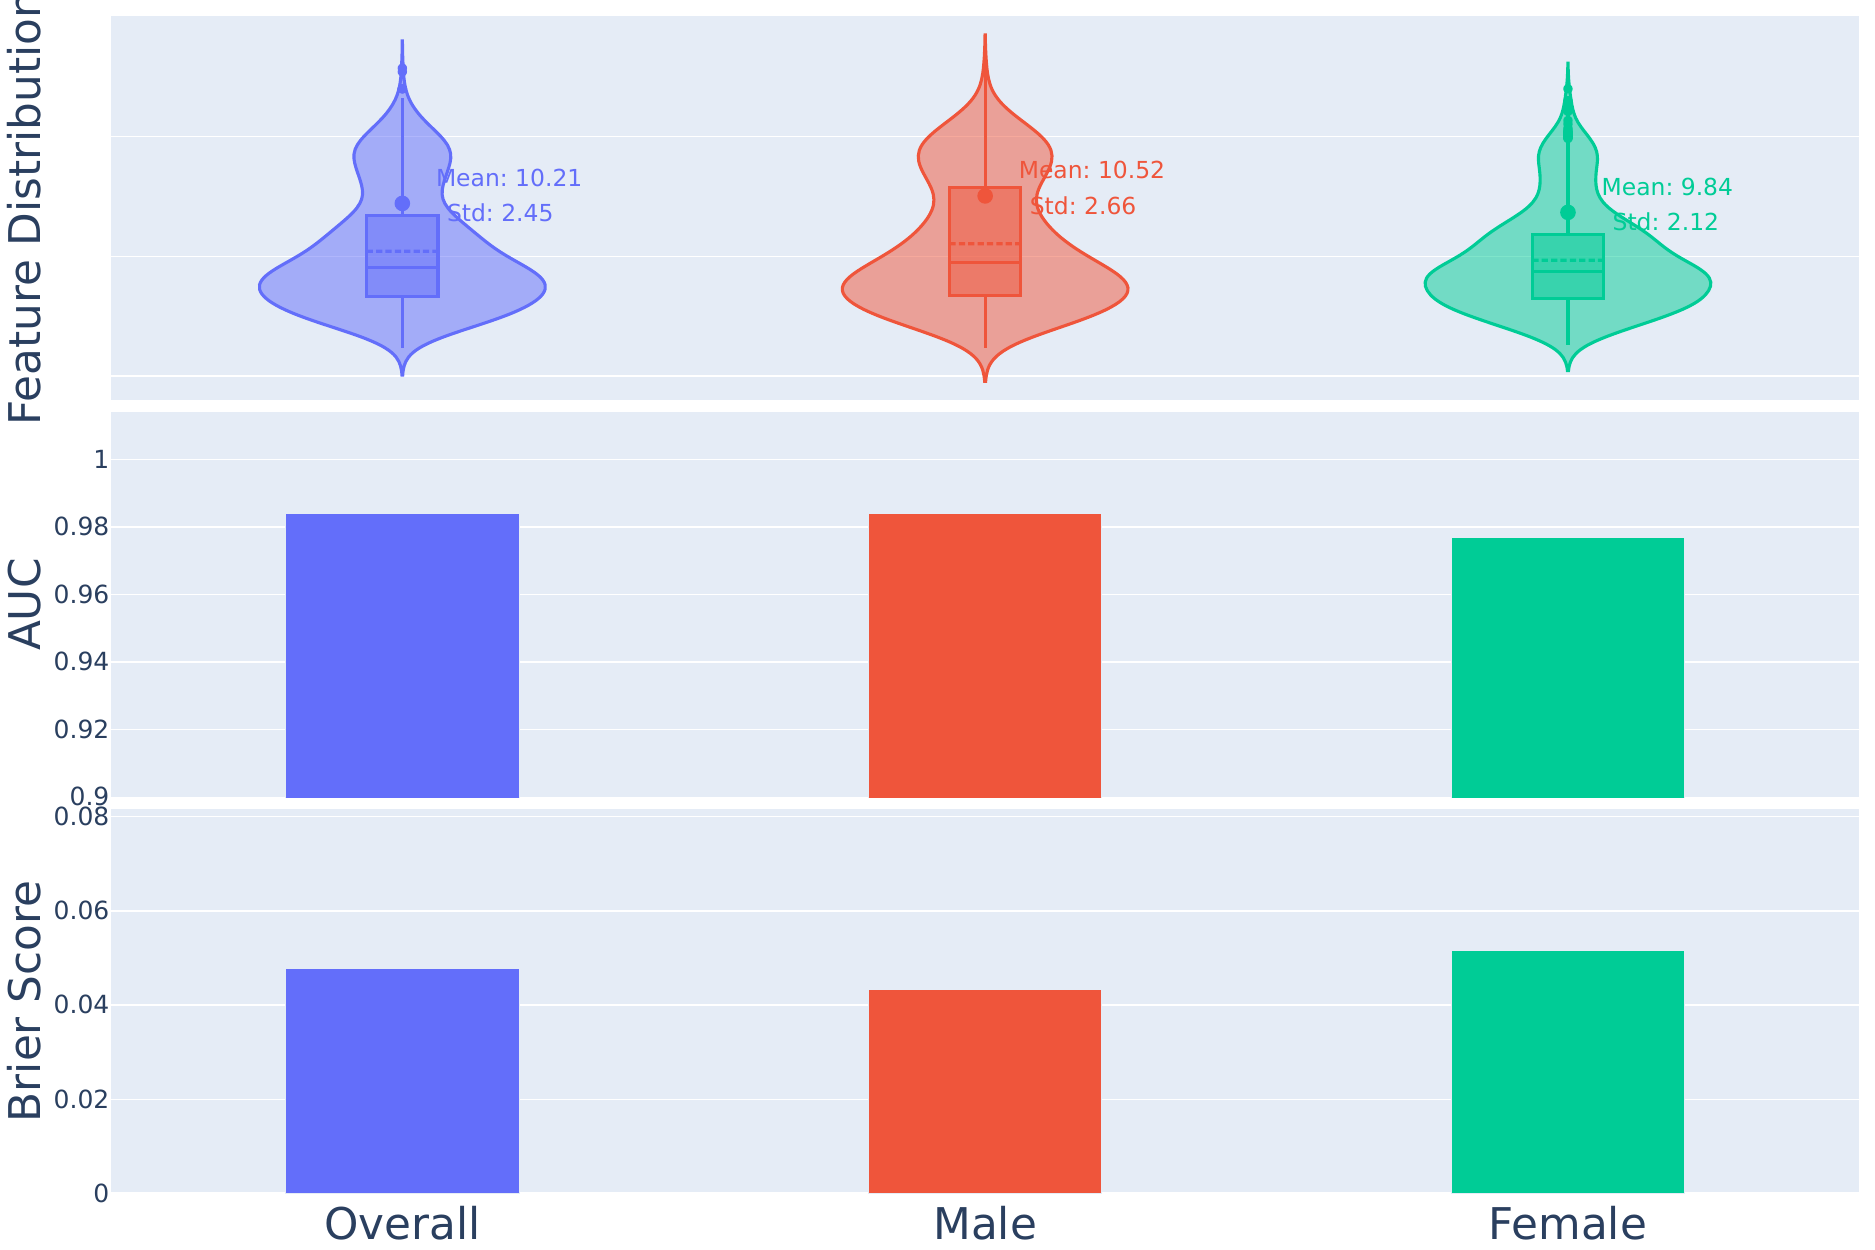}
        \caption{Glasses Detection on Gender}
        \label{fig:combination_pe_vit}
    \end{subfigure} \\
    \caption{Combination of feature distribution, AUC, and Brier Score with EfficientNet for Glasses detection on the \textbf{FairFace dataset} across three attributes: Age, Skin Color, and Gender.}
    \label{fig_fairface}
\end{figure}
